# Supplementary material for: Exploring particle dynamics in flowing complex fluids using differential dynamic microscopy
Source: arXiv:2107.12946 ancillary file (2021-07-27)
Supplement: Supplementary file 1 [file echoDDM_ESI.pdf]

# Supplementary Information: Exploring particle dynamics in flowing complex fluids using differential dynamic microscopy

James A. Richards,\* Vincent A. Martinez, and Jochen Arlt

This supplementary information contains four sections, providing additional information to further support the main text. Section S1 details the additional terms in the ISF for flow-DDM and the  $q$ -dependent fitting. In §S2 we compare the parallel and perpendicular sectors of the DICF in echo-DDM for a dilute colloid; and, in §S3 the fitting parameters for the ISF in echo-DDM of a silicone oil emulsion are presented. Finally, in §S4 images of the diluted emulsion are presented.

## S1 Flow-DDM details

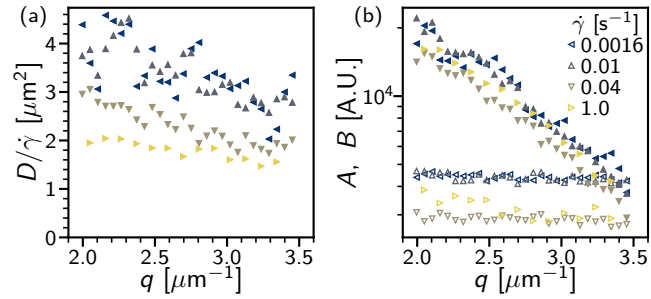

**Fig. S1** Lengthscale dependence of flow-DDM fitting. (a) Diffusivity normalised by applied shear rate,  $D/\dot{\gamma}$ , as a function of spatial Fourier mode,  $q$ , over averaging range used. For  $\dot{\gamma}$ , see legend in (b). (b) Signal strength,  $A(q)$  (filled), and noise term,  $B(q)$  (open symbols). See inset legend for  $\dot{\gamma}$

In flow-DDM residual impacts of the flow velocity may remain in the drift-corrected DICF,  $\bar{g}$ , even in the perpendicular sector. Following Ref.<sup>1</sup>, to ensure that microscopic diffusive dynamics,  $f_D = \exp(-Dq^2\tau)$ , are measured from the ISF,  $\bar{f}^\perp$ , we must consider additional terms encompassing these residual effects:

$$\bar{f}(\vec{q}, \tau) = f_D \cdot f_{FS} \cdot f_{\Delta v}. \quad (\text{S1})$$

By estimating these terms, or bounds for these terms, alongside  $f_D$  we can establish that the timescales for decorrelation due to flow effects are above that of the timescale due to microscopic rearrangements,  $t_D$ , and hence that decorrelation of the measured ISF is related to  $t_D$ .

Equation S1 includes a finite size term,  $f_{FS}$ , as particles leave the field of view with the flow. The rate is set by the speed,  $v$ , and the length of the image in the flow direction,  $L$ :

$$f_{FS} = \max\left(1 - \frac{v\tau}{L}\right). \quad (\text{S2})$$

The velocity,  $v$ , is measured in calculating  $\bar{g}$ . It can therefore be separately calculated and in all results it is found to be negligible. The final term,  $f_{\Delta v}$ , is due to the velocity distribution. After drift correction  $\Delta v$  leaves a range of residual velocities in the flow direction. This effect is then highly direction dependent. We minimise the impact of  $\Delta v$  by taking a narrow sector perpendicular to the flow direction, where

$$f_{\Delta v}^\perp = \text{Si}(vq\theta\tau)/(vq\theta\tau). \quad (\text{S3})$$

Here Si is the sine integral, which decays monotonically. In the perpendicular sector alone the impact of a velocity distribution cannot be robustly distinguished from diffusive behaviour. We therefore use the direction dependence and simultaneously fit a perpendicular and an adjacent sector where

$$f_{\Delta v}^{\perp\parallel} = [\text{Si}(3q\Delta v\tau\theta) - \text{Si}(q\Delta v\tau\theta)]/(2q\Delta v\tau\theta), \quad (\text{S4})$$

and the impact of  $\Delta v$  is greater. As  $\Delta v$  is in principle fixed for our imaging and flow geometry we fit a single  $\Delta v$  over a  $q$  range of  $2.0\mu\text{m}^{-1}$  to  $3.5\mu\text{m}^{-1}$ , with  $D(q)$  and for each sector  $\{A(q), B(q)\}$ . The extracted  $\Delta v$  is found to be negligible. We report the full  $q$  dependence of the parameters in Fig. S1 for a selected range of shear rates,  $\dot{\gamma}$ . At low rates,  $\dot{\gamma} < 1\text{s}^{-1}$  a weak  $q$  dependence may exist, although any trend is comparable to the noise. We therefore treat the behaviour as diffusive in the main text, although experiments probing a broader

$q$  range may allow flow-DDM to investigate this aspect. The signal strength,  $A(q)$  [Fig. S1(b) (filled symbols)], is independent of the applied rate, as for echo-DDM of oscillatory shear.

## S2 Parallel sector echo-DDM

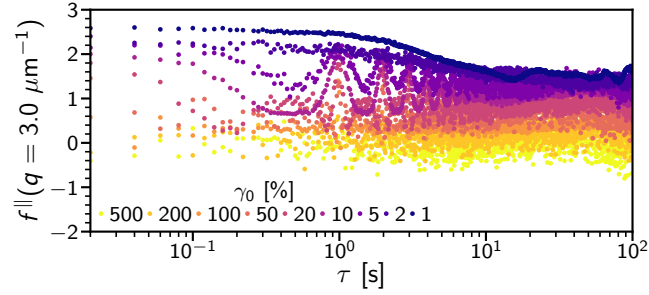

**Fig. S2** Parallel sector of echo-DDM for a dilute diffusing colloidal suspension. Sector width  $\theta = 3^\circ$  in flow direction. Symbols, reconstructed ISF,  $f^{\parallel}(\tau)$  at  $q = 3\mu\text{m}^{-1}$ , equivalent perpendicular sector in Fig. 3(c). Symbols, data at applied strain amplitude,  $\gamma_0$  (see inset legend), shift applied to  $f^{\parallel}$  from 0 to 2.4.

In the main text, Section. 4.1, we present echo-DDM of a dilute diffusing colloid undergoing oscillatory flow using the perpendicular sector, Fig. 3. In the reconstructed ISF,  $f^{\perp}$  in Fig. 3(c), the impact of flow is negligible in the perpendicular sector for strain amplitudes,  $\gamma_0 \leq 20\%$ . Above this the full ISF becomes modulated by the oscillation frequency and only  $f_{\text{echo}}^{\perp}$  recovers the diffusive dynamics. Echo-DDM then fails at larger  $\gamma_0 > 100\%$ , where the peak of the sample returning to the original bulk location cannot be recovered. It should be stressed that selecting the peak ISF values is not the only mechanism to reduce the impact of the oscillatory flow in  $f_{\text{echo}}^{\perp}$ : the impact has been substantially reduced already by selection of the perpendicular sector. The importance of this reduced analysis of the DICF can be shown by comparison of Fig. 3(c) with the equivalent in the parallel sector, Fig. S2. To reconstruct the ISF,  $g^{\parallel} = A(1 - f^{\parallel}) + B$ ,  $B(q)$  uses  $g^{\parallel}(t_f)$  and  $A(q)$  is extracted from the long time limit, as direct fitting of a parameterised ISF is not possible. In the sector parallel to the flow direction the ISF,  $f^{\parallel}$  strongly modulated at only  $\gamma_0 = 5\%$ , with narrowing peaks from  $\geq 10\%$  (purple). At an applied strain of 50% the ISF is difficult to even trace (orange), demonstrating the impact of selecting the perpendicular sector to reduce the impact of flow.

## S3 ISF fitting parameters

### S3.1 Conversion of DICF into ISF

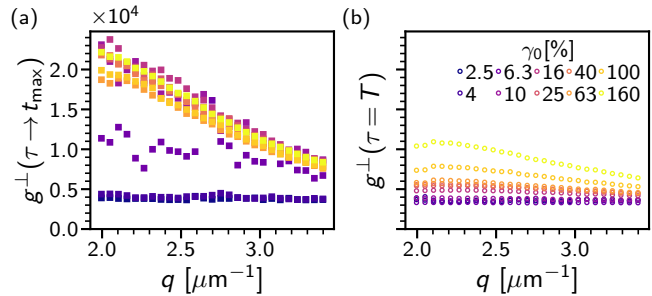

**Fig. S3** DICF limits for echo-DDM of a silicone oil emulsion. (a) Long-time limit of perpendicular sector DICF average of  $g_{\text{echo}}^{\perp}$  from  $t = 90$  s to 100 s with changing strain amplitude, see inset legend in (b). Shown over extended  $q$  range,  $2.0\mu\text{m}^{-1}$  to  $3.5\mu\text{m}^{-1}$ , with  $2.0\mu\text{m}^{-1}$  to  $2.4\mu\text{m}^{-1}$  for averaging. DICF values in arbitrary units. (b) Short-time limit from  $g^{\perp}(t_f)$ , strain amplitudes in legend.

In a conventional approach to fitting at each  $q$  the DICF,  $g(\tau)$ , would be fitted directly with  $A$  and  $B$  as fit parameters alongside the parameterised ISF. This approach works where the short-time [ $g(\tau \rightarrow 0) = B$ ] and long-time [ $g(\tau \rightarrow \infty) - B = A$ ] plateaus are well captured or if the form of the ISF is well-known to allow extrapolation (e.g. diffusion). For oscillatory flow of a concentrated silicone emulsion these conditions do not hold, Fig. 4(a). We must therefore reconstruct the ISF from the DICF before fitting a parameterised ISF. To recover the fully correlated [ $B(q)$ ] and fully decorrelated [ $A(q) + B(q)$ ] DICF values we consider the short-time ( $t_f$ ) and long-time ( $\sim t_{\text{max}}$ ) values as a function of strain amplitude, Fig. S3. The values of  $A(q)$  and  $B(q)$  do not depend on strain amplitude and this lack of impact for flow is seen in a dilute colloid, Fig. 3(d). Changes in the DICF limits within experimental timescales are therefore due to changes in the ISF. For small strain amplitudes ( $\gamma_0 \leq 10\%$ ),  $g^{\perp}(\tau \rightarrow t_{\text{max}})$  increases. The system therefore cannot be assumed to fully decorrelate at these strains, while at high strains the DICF limit becomes independent of  $\gamma_0$ . To reconstruct the DICF  $g^{\perp}(\tau \rightarrow t_{\text{max}}, \gamma_0 = 160\%)$  is used to

determine  $A(q)$  for  $\gamma_0 \leq 10\%$ . Similarly, at high strains,  $\gamma_0 \geq 40\%$ , the short-time behaviour becomes strain dependent. The system begins to decorrelate before the first frame delay. For  $B(q)$  the low-strain correlated value is then used,  $g^\perp(\tau = t_f, \gamma_0 = 2.5\%)$ . Note that  $\tau = t_f$  is only used in ISF reconstruction and not for fitting of the parameterised ISF.

### S3.2 ISF fitting parameters

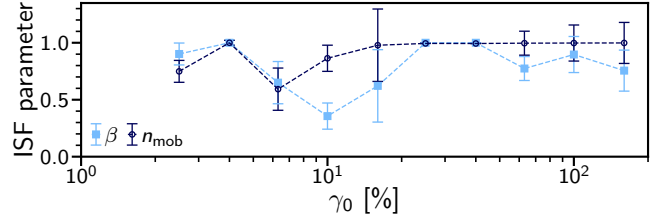

**Fig. S4** Intermediate scattering function functional form. Parameters from stretched exponential [ $\beta$  in Eq. S5, light (blue) squares] and non-ergodic diffusive form [mobile fraction,  $n_{\text{mob}}$ , in Eq. S6, dark (blue) circles] as a function of applied strain amplitude,  $\gamma_0$ . Average and error (standard deviation) taken over  $q = 2.0 \mu\text{m}^{-1}$  to  $2.3 \mu\text{m}^{-1}$ .

Near the onset of rearrangements the form of the ISF is not a diffusive decorrelation, the system begins to decorrelate from the first oscillation cycle, but a clear decorrelated plateau ( $f_{\text{echo}}^\perp = 0$ ) is not reached two decades later in  $\tau$ , Fig. 5. To capture this behaviour we fit either a stretched exponential,

$$f_{\text{echo}}^\perp = \exp \left[ - \left( Dq^2 \tau \right)^\beta \right], \quad (\text{S5})$$

or a non-ergodic ISF, where only a proportion of the particles are mobile:

$$f_{\text{echo}}^\perp = n_{\text{mob}} \exp \left( - Dq^2 \tau \right) + (1 - n_{\text{mob}}). \quad (\text{S6})$$

This decreases from  $f = 1$  to a non-zero plateau ( $f = 1 - n_{\text{mob}}$ ). We fit both functions over all  $\gamma_0$ , allowing  $0 < n_{\text{mob}}, \beta \leq 1$ . In the main text we report the extracted diffusion coefficient, Fig. 5(b) [inset], and in Fig. S4 the corresponding modification to the ISF function is shown, Eqs. S5 and S6. At the smallest strains,  $\gamma_0 \leq 2.5\%$ , no decorrelation is observed within experimental timescales and  $n_{\text{mob}}$  becomes poorly defined and we report only  $D_{\text{osc}}$  from a stretched exponential which captures a decorrelation time  $\gg t_{\text{max}}$ . At  $\gamma_0 = 6.3$  to 16% both  $n_{\text{mob}}$  and  $\beta$  decrease below 1. As decorrelation is no longer a simple exponential decay, the dynamics are heterogeneous, with rearrangement dynamics over an oscillation cycle and over timescales beyond the experimental window. At  $\gamma_0 > 16\%$  the decay returns to a simple exponential, although this fit uses only a small number of data points. As the number of  $\tau$  with  $f_{\text{echo}}^\perp > 0$  decreases the stretched exponent becomes ill-defined and we report only the diffusivity from Eq. S6 for  $\gamma_0 > 25\%$ .

## S4 Emulsion dilution

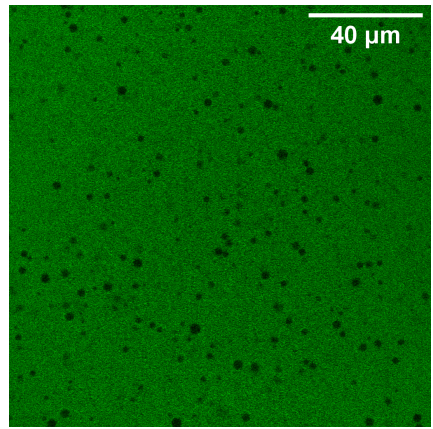

**Fig. S5** Diluted emulsion in background solvent imaged at high magnification (63 $\times$ ) using confocal microscopy, see scale bar

In the silicone-oil emulsion an excess of SDS can cause a depletion interaction that leads to a thixotropic response and strong shear banding<sup>2</sup>. Although we see shear localisation, it should be noted that our system is not of this type. This is evidenced by diluting the concentrated emulsion in additional background solvent, Fig. S5. With the presence of attraction and thixotropy, distinct clusters of

droplets can be seen in microscopy, instead droplets are dispersed across the sample. Further evidence of the lack of thixotropy is seen in the intracycle velocity, as upon reversal the system rapidly returns to an elastic solid with a low degree of shear localisation, Fig. 8.

## References

- 1 J. A. Richards, V. A. Martinez and J. Arlt, *Soft Matter*, 2021, **17**, 3945–3953.
- 2 L. Bécu, S. Manneville and A. Colin, *Phys. Rev. Lett.*, 2006, **96**, 138302.
